# Supplementary material for: Piecewise Robust Barrier Tubes for Nonlinear Hybrid Systems with Uncertainty
Source: arXiv:1907.11514 source file (2019-07-25)
Supplement: Supplementary file 1 [file appendix.tex]

%\appendix%
%\section{Appendix}
\subsection{Proof of Theorem~\ref{thrmhandeltrans}}\label{proof_handel}
\begin{proof}
	Since $\lambda_{\vec{\alpha}}$'s are all nonnegative and $\epsilon_1$ is positive, it is easy prove that for any $\vec{x}\in \Init$, $B(\vec{x})  \equiv \sum_{|\vec{\alpha}|\leq M_1} \lambda_{\vec{\alpha}}p_1^{\alpha_1}\cdots p_{m_1}^{\alpha_{m_1}} + \epsilon_1 > 0$, therefore the formula~\ref{eq4} implies the formula~\eqref{eq1} in Theorem~\ref{thrmbarrer} holds. Likewise, we can prove that the formula~\ref{eq5} and \ref{eq6} imply the formula~\ref{eq2} and \ref{eq3} respectively. Therefore, the system is guaranteed to be safe.
\end{proof}

\subsection{Proof of Theorem~\ref{thrmtube}}\label{sec:prove_tube}	
\begin{proof}
	According to Theorem~\ref{thrmbarrer}, it is easy to prove that for every $B_i(\vx)\in BT$, $B_i(\vx)$ is an invariant of \sys in $E$. Hence we have $Flow_{\vec{f}}(\Init) \cap E \subseteq \{\vec{x}\in \R^n \mid B_i(\vec{x})>0 \} \cap E$. Then, $Flow_{\vec{f}}(\Init) \cap E \subseteq \Omega \cap E$. 
\end{proof}
